# Supplementary material for: Assessment of machine learning methods for state-to-state approaches
Source: arXiv:2104.01042 source file (2021-04-02)
Supplement: Supplementary file 1 [file AppendixRelaxationRegression.tex]

\newpage
\section{Appendix: relaxation terms regression}\label{AppendixRelaxation}
% http://blog.pengyifan.com/the-best-way-to-place-figures-side-by-side-in-latex/
% Relaxation source term (DR)
\begin{figure}[!ht]
%%
%\begin{minipage}[b]{0.45\textwidth}
%    \includegraphics[width=\textwidth]{figs/SourceTerm/regression_MO_KR_DR}\\Ker%nelRidge
%    %\caption{KernelRidge}
%  \end{minipage}
%  \hfill
%  \begin{minipage}[b]{0.45\textwidth}
%    \includegraphics[width=\textwidth]{figs/SourceTerm/regression_MO_SVR_DR}\\Su%pportVectorMachine
%    %\caption{SupportVectorMachine}
%  \end{minipage}
%%
\begin{subfigure}{0.45\textwidth}
\includegraphics[scale=0.5]{figs/SourceTerm/regression_MO_KR_DR}
\caption{KernelRidge}
\label{fig:KR_DR}
\end{subfigure}
\begin{subfigure}{0.45\textwidth}
\includegraphics[scale=0.5]{figs/SourceTerm/regression_MO_SVR_DR}
\caption{SupportVectorMachine}
\label{fig:SVR_DR}
\end{subfigure}
\\
%%
%\begin{minipage}[b]{0.45\textwidth}
%    \includegraphics[width=\textwidth]{figs/SourceTerm/regression_MO_RF_DR}\\k-N%earest Neighbour
%    %\caption{k-Nearest Neighbour}
%  \end{minipage}
%  \hfill
%  \begin{minipage}[b]{0.45\textwidth}
%    \includegraphics[width=\textwidth]{figs/SourceTerm/regression_MO_DT_DR}\\Gau%ssianProcess
%    %\caption{GaussianProcess}
%  \end{minipage}
  %%
\begin{subfigure}{0.45\textwidth}
\includegraphics[scale=0.5]{figs/SourceTerm/regression_MO_kNN_DR}
\caption{k-Nearest Neighbour}
\label{fig:kNN_DR}
\end{subfigure}
\begin{subfigure}{0.45\textwidth} %FIXME
\includegraphics[scale=0.5]{figs/SourceTerm/regression_MO_RF_DR}
\caption{GaussianProcess}
\label{fig:GP_DR}
\end{subfigure}
\\
%%
%\begin{minipage}[b]{0.45\textwidth}
%    \includegraphics[width=\textwidth]{figs/SourceTerm/regression_MO_DT_DR}\\Dec%isionTree
%    %\caption{DecisionTree}
%  \end{minipage}
%  \hfill
%  \begin{minipage}[b]{0.45\textwidth}
%    \includegraphics[width=\textwidth]{figs/SourceTerm/regression_MO_RF_DR}\\Ran%domForest
%    %\caption{RandomForest}
%  \end{minipage}
%%
\begin{subfigure}{0.45\textwidth}
\includegraphics[scale=0.5]{figs/SourceTerm/regression_MO_DT_DR}
\caption{DecisionTree}
\label{fig:DT_DR}
\end{subfigure}
\begin{subfigure}{0.45\textwidth}
\includegraphics[scale=0.5]{figs/SourceTerm/regression_MO_RF_DR}
\caption{RandomForest}
\label{fig:RF_DR}
\end{subfigure}
\\
%%
%\begin{minipage}[b]{0.45\textwidth}
%    \includegraphics[width=\textwidth]{figs/SourceTerm/regression_MO_ET_DR}\\Ext%raTrees
%    %\caption{ExtraTrees}
%  \end{minipage}
%  \hfill
%  \begin{minipage}[b]{0.45\textwidth}
%    \includegraphics[width=\textwidth]{figs/SourceTerm/regression_MO_GB_DR}\\Gra%dientBoosting
%    %\caption{GradientBoosting}
%  \end{minipage}
%%  
\begin{subfigure}{0.45\textwidth}
\includegraphics[scale=0.5]{figs/SourceTerm/regression_MO_ET_DR}
\caption{ExtraTrees}
\label{fig:ET_DR}
\end{subfigure}
\begin{subfigure}{0.45\textwidth}
\includegraphics[scale=0.5]{figs/SourceTerm/regression_MO_GB_DR}
\caption{GradientBoosting}
\label{fig:GB_DR}
\end{subfigure}
\end{figure}
\newpage
\begin{figure}[!ht]
\ContinuedFloat
%
%%
%\begin{minipage}[b]{0.45\textwidth}
%    \includegraphics[width=\textwidth]{figs/SourceTerm/regression_MO_HGB_DR}\\Hi%stGradientBoosting
%    %\caption{HistGradientBoosting}
%  \end{minipage}
%  \hfill
%  \begin{minipage}[b]{0.45\textwidth}
%    \includegraphics[width=\textwidth]{figs/SourceTerm/regression_MO_MLP_DR}\\Mu%lti-layer Perceptron
%    %\caption{Multi-layer Perceptron}
%  \end{minipage}
%%  
\begin{subfigure}{0.45\textwidth}
\includegraphics[scale=0.5]{figs/SourceTerm/regression_MO_HGB_DR}
\caption{HistGradientBoosting}
\label{fig:HGB_DR}
\end{subfigure}
\begin{subfigure}{0.45\textwidth}
\includegraphics[scale=0.5]{figs/SourceTerm/regression_MO_MLP_DR}
\caption{Multi-layer Perceptron}
\label{fig:MLP_DR}
\end{subfigure}
\caption{Relaxation terms for DR process regression.}
\label{fig:relax_comparison_DR}
\end{figure}
\newpage
%
% Relaxation source term (VT)
\begin{figure}[!ht]
%
%\begin{minipage}[b]{0.45\textwidth}
%    \includegraphics[width=\textwidth]{figs/SourceTerm/regression_MO_KR_VT}\\Ker%nelRidge
%    %\caption{KernelRidge}
%  \end{minipage}
%  \hfill
%  \begin{minipage}[b]{0.45\textwidth}
%    \includegraphics[width=\textwidth]{figs/SourceTerm/regression_MO_SVR_VT}\\Su%pportVectorMachine
%    %\caption{SupportVectorMachine}
%  \end{minipage}
  %%
\begin{subfigure}{0.45\textwidth}
\includegraphics[scale=0.5]{figs/SourceTerm/regression_MO_KR_VT}
\caption{KernelRidge}
\label{fig:KR_VT}
\end{subfigure}
\begin{subfigure}{0.45\textwidth}
\includegraphics[scale=0.5]{figs/SourceTerm/regression_MO_SVR_VT}
\caption{SupportVectorMachine}
\label{fig:_SVR_VT}
\end{subfigure}
\\
%%
%\begin{minipage}[b]{0.45\textwidth}
%    \includegraphics[width=\textwidth]{figs/SourceTerm/regression_MO_kNN_VT}\\k-%Nearest Neighbour
%    %\caption{k-Nearest Neighbour}
%  \end{minipage}
%  \hfill
%  \begin{minipage}[b]{0.45\textwidth}
%    \includegraphics[width=\textwidth]{figs/SourceTerm/regression_MO_GP_VT}\\Gau%ssianProcess
%    %\caption{GaussianProcess}
%  \end{minipage}
  %%
\begin{subfigure}{0.45\textwidth}
\includegraphics[scale=0.5]{figs/SourceTerm/regression_MO_kNN_VT}
\caption{k-Nearest Neighbour}
\label{fig:kNN_VT}
\end{subfigure}
\begin{subfigure}{0.45\textwidth}
\includegraphics[scale=0.5]{figs/SourceTerm/regression_MO_GP_VT}
\caption{GaussianProcess}
\label{fig:GP_VT}
\end{subfigure}
\\
%%
%\begin{minipage}[b]{0.45\textwidth}
%    \includegraphics[width=\textwidth]{figs/SourceTerm/regression_MO_DT_VT}\\Dec%isionTree
%    %\caption{DecisionTree}
%  \end{minipage}
%  \hfill
%  \begin{minipage}[b]{0.45\textwidth}
%    \includegraphics[width=\textwidth]{figs/SourceTerm/regression_MO_RF_VT}\\Ran%domForest
%    %\caption{RandomForest}
%  \end{minipage}
  %%
\begin{subfigure}{0.45\textwidth}
\includegraphics[scale=0.5]{figs/SourceTerm/regression_MO_DT_VT}
\caption{DecisionTree}
\label{fig:DT_VT}
\end{subfigure}
\begin{subfigure}{0.45\textwidth}
\includegraphics[scale=0.5]{figs/SourceTerm/regression_MO_RF_VT}
\caption{RandomForest}
\label{fig:RF_VT}
\end{subfigure}
\\
%%
%\begin{minipage}[b]{0.45\textwidth}
%    \includegraphics[width=\textwidth]{figs/SourceTerm/regression_MO_ET_VT}\\Ext%raTrees
%    %\caption{ExtraTrees}
%  \end{minipage}
%  \hfill
%  \begin{minipage}[b]{0.45\textwidth}
%    \includegraphics[width=\textwidth]{figs/SourceTerm/regression_MO_GB_VT}\\Gra%dientBoosting
%    %\caption{GradientBoosting}
%  \end{minipage}
  %%
\begin{subfigure}{0.45\textwidth}
\includegraphics[scale=0.5]{figs/SourceTerm/regression_MO_ET_VT}
\caption{ExtraTrees}
\label{fig:ET_VT}
\end{subfigure}
\begin{subfigure}{0.45\textwidth}
\includegraphics[scale=0.5]{figs/SourceTerm/regression_MO_GB_VT}
\caption{GradientBoosting}
\label{fig:GB_VT}
\end{subfigure}
\end{figure}
\newpage
\begin{figure}[!ht]
\ContinuedFloat
%
%%
%\begin{minipage}[b]{0.45\textwidth}
%    \includegraphics[width=\textwidth]{figs/SourceTerm/regression_MO_HGB_VT}\\Hi%stGradientBoosting
%    %\caption{HistGradientBoosting}
%  \end{minipage}
%  \hfill
%  \begin{minipage}[b]{0.45\textwidth}
%    \includegraphics[width=\textwidth]{figs/SourceTerm/regression_MO_MLP_VT}\\Mu%lti-layer Perceptron
%    %\caption{Multi-layer Perceptron}
%  \end{minipage}
  %%
\begin{subfigure}{0.45\textwidth}
\includegraphics[scale=0.5]{figs/SourceTerm/regression_MO_HGB_VT}
\caption{HistGradientBoosting}
\label{fig:HGB_VT}
\end{subfigure}
\begin{subfigure}{0.45\textwidth}
\includegraphics[scale=0.5]{figs/SourceTerm/regression_MO_MLP_VT}
\caption{Multi-layer Perceptron}
\label{fig:MLP_VT}
\end{subfigure}
\caption{Relaxation terms for VT exchange process regression.}
\label{fig:relax_comparison_VT}
\end{figure}
\newpage
%
% Relaxation source term (VV)
\begin{figure}[!ht]
%
%%
%\begin{minipage}[b]{0.45\textwidth}
%    \includegraphics[width=\textwidth]{figs/SourceTerm/regression_MO_KR_VV}\\Ker%nelRidge
%    %\caption{KernelRidge}
%  \end{minipage}
%  \hfill
%  \begin{minipage}[b]{0.45\textwidth}
%    \includegraphics[width=\textwidth]{figs/SourceTerm/regression_MO_SVR_VV}\\Su%pportVectorMachine
%    %\caption{SupportVectorMachine}
%  \end{minipage}
  %%
\begin{subfigure}{0.45\textwidth}
\includegraphics[scale=0.5]{figs/SourceTerm/regression_MO_KR_VV}
\caption{KernelRidge}
\label{fig:KR_VV}
\end{subfigure}
\begin{subfigure}{0.45\textwidth}
\includegraphics[scale=0.5]{figs/SourceTerm/regression_MO_SVR_VV}
\caption{SupportVectorMachine}
\label{fig:_SVR_VV}
\end{subfigure}
\\
%%
%\begin{minipage}[b]{0.45\textwidth}
%    \includegraphics[width=\textwidth]{figs/SourceTerm/regression_MO_kNN_VV}\\k-%Nearest Neighbour
%    %\caption{k-Nearest Neighbour}
%  \end{minipage}
%  \hfill
%  \begin{minipage}[b]{0.45\textwidth}
%    \includegraphics[width=\textwidth]{figs/SourceTerm/regression_MO_GP_VV}\\Gau%ssianProcess
%    %\caption{GaussianProcess}
%  \end{minipage}
%%
\begin{subfigure}{0.45\textwidth}
\includegraphics[scale=0.5]{figs/SourceTerm/regression_MO_kNN_VV}
\caption{k-Nearest Neighbour}
\label{fig:kNN_VV}
\end{subfigure}
\begin{subfigure}{0.45\textwidth}
\includegraphics[scale=0.5]{figs/SourceTerm/regression_MO_GP_VV}
\caption{GaussianProcess}
\label{fig:GP_VV}
\end{subfigure}
\\
%%
%\begin{minipage}[b]{0.45\textwidth}
%    \includegraphics[width=\textwidth]{figs/SourceTerm/regression_MO_DT_VV}\\Dec%isionTree
%    %\caption{DecisionTree}
%  \end{minipage}
%  \hfill
%  \begin{minipage}[b]{0.45\textwidth}
%    \includegraphics[width=\textwidth]{figs/SourceTerm/regression_MO_RF_VV}\\Ran%domForest
%    %\caption{RandomForest}
%  \end{minipage}
%%
\begin{subfigure}{0.45\textwidth}
\includegraphics[scale=0.5]{figs/SourceTerm/regression_MO_DT_VV}
\caption{DecisionTree}
\label{fig:DT_VV}
\end{subfigure}
\begin{subfigure}{0.45\textwidth}
\includegraphics[scale=0.5]{figs/SourceTerm/regression_MO_RF_VV}
\caption{RandomForest}
\label{fig:RF_VV}
\end{subfigure}
\\
%%
%\begin{minipage}[b]{0.45\textwidth}
%    \includegraphics[width=\textwidth]{figs/SourceTerm/regression_MO_ET_VV}\\Ext%raTrees
%    %\caption{ExtraTrees}
%  \end{minipage}
%  \hfill
%  \begin{minipage}[b]{0.45\textwidth}
%    \includegraphics[width=\textwidth]{figs/SourceTerm/regression_MO_GB_VV}\\Gra%dientBoosting
%    %\caption{GradientBoosting}
%  \end{minipage}
%%
\begin{subfigure}{0.45\textwidth}
\includegraphics[scale=0.5]{figs/SourceTerm/regression_MO_ET_VV}
\caption{ExtraTrees}
\label{fig:ET_VV}
\end{subfigure}
\begin{subfigure}{0.45\textwidth}
\includegraphics[scale=0.5]{figs/SourceTerm/regression_MO_GB_VV}
\caption{GradientBoosting}
\label{fig:GB_VV}
\end{subfigure}
\end{figure}
\newpage
\begin{figure}[!ht]
\ContinuedFloat
%
%%
%\begin{minipage}[b]{0.45\textwidth}
%    \includegraphics[width=\textwidth]{figs/SourceTerm/regression_MO_HGB_VV}\\Hi%stGradientBoosting
%    %\caption{HistGradientBoosting}
%  \end{minipage}
%  \hfill
%  \begin{minipage}[b]{0.45\textwidth}
%    \includegraphics[width=\textwidth]{figs/SourceTerm/regression_MO_MLP_VV}\\Mu%lti-layer Perceptron
%    %\caption{Multi-layer Perceptron}
%  \end{minipage}
%%
\begin{subfigure}{0.45\textwidth}
\includegraphics[scale=0.5]{figs/SourceTerm/regression_MO_HGB_VV}
\caption{HistGradientBoosting}
\label{fig:HGB_VV}
\end{subfigure}
\begin{subfigure}{0.45\textwidth}
\includegraphics[scale=0.5]{figs/SourceTerm/regression_MO_MLP_VV}
\caption{Multi-layer Perceptron}
\label{fig:MLP_VV}
\end{subfigure}
\caption{Relaxation terms for VV exchange process regression.}
\label{fig:relax_comparison_VV}
\end{figure}
